# Supplementary material for: Point absorbers in Advanced LIGO
Source: arXiv:2101.05828 source file (2021-03-25)
Supplement: Supplementary file 1 [file appendix.tex]

\section{Derivations}

\subsection{Power-recycling gain v loss}

The scatter out of the TEM00 mode is approximately proportional to the square of magnitude of  the wavefront distortion.

We plot scatter into HOM as a function of point absorber power  the loss from the TEM00 with uniform absorption.

\begin{eqnarray}
    L_{00}\left(t\right) & = & 1 - \left|\langle U_{00} \left|W_{u}\left(x,y,t\right)\right|U_{00} \rangle\right|^2 \\
    & = & 1 - \left| \iint_{-\infty}^{\infty} \mathrm{e}^{\left(-2\left(\frac{r}{w}\right)^2\right)} \, \mathrm{e}^{\left( \mathrm{i}\,k\,W_u(x,y,t)\right)} \right|^2 \\
    & \approx NO & \left|k\,  \iint_{-\infty}^{\infty} \mathrm{e}^{\left(-2\left(\frac{r}{w}\right)^2\right)} \,P\,V_u(x,y,t) \right|^2\\
    & = & c_{00}\, P^2
\end{eqnarray}

\begin{equation}
    S_{ij}\left(t\right) = \langle U_{ij} \left|W_{pt}\left(t\right)\right|U_{00} \rangle
\end{equation}

\begin{equation}
    G_{\mathrm{PRG}}(P_{\mathrm{in}}) = G_{0} - dG\,P_{\mathrm{in}}^2 
\end{equation}

We then solve for the apparent loss, $L_{arm}$, and then for the power-dependent scatter coefficient, $c_{00}$.

\section{Tables of measurements}

% HWS data
\begin{table*}[ht]
\centering
\begin{tabular}{| l | c | c | c | c | c |}
\hline
{\bf Optic name} & {\bf Location} & {\bf Uniform} & \multicolumn{2}{c|}{\textbf{Point absorbers}} & {\bf Residual RMS} \\
  &   & {\bf absorp. (ppb) } & \multicolumn{2}{l|}{}  & {\bf OPD at \SI{200}{\kilo\watt} }\\
\hline
  &   & & {\bf Coords. (mm)} & {\bf MAD ($\mu$m)}  & \\
\hline
\hline
ITM-03 & H1-ITMX [O2 only] & 150 $\pm$ 100 & [+25,-25]* & 40 & \SI{5}{\nano\meter} \\
 & &  & [-25,-25]* & 38 &  \\
\hline
ITM-04 & H1-ITMX [O3 only] & 150 &  &  & \SI{5}{\nano\meter} \\
\hline
ITM-07 & H1-ITMY [O2/O3] & 150 & [+25,-25]* & 40 & \SI{5}{\nano\meter} \\
 & &  & [-25,-25]* & 38 &  \\
 & &  & [-02,+11]* & 15 &  \\
 & &  & [+05,+18]* & 17 &  \\
 & &  & [+11,-54]* & 11 &  \\
\hline
\end{tabular}
\label{tab:HWS_measurements}
\caption{HWS measurement summary \textcolor{red}{currently contains example data}. Asterisks on coordinates indicate HWS coordinate system (for instances in which we were unable to calibrate the relative positions of the HWS and optic coordinate systems.). \textcolor{red}{do fits with transient data set - 4 or 5 times at increasing intervals. Also, have to remove obviously flawed gradient measurements.}}
\end{table*}

% PCI data

\begin{table*}[ht]
\centering
\begin{tabular}{| l | c | c | c | c | p{4cm} | c |}
\hline
{\bf Name } & {\bf Meas.}  & {\bf Noise floor} &  {\bf \# points above }   & {\bf Max.}          & {\bf Comments} & {\bf History }\\
            & {\bf diam (mm)}  &  {\bf (ppm)}       &   {\bf noise floor }  & {\bf absorp. (ppm)} &                & \\
\hline
\hline
ITM03 & 60 & $\approx$ 50  & 4 & $\approx$ 1000 & Further measurement with \SI{60}{\micro\meter} beam max  $\approx$ 20000 ppm & H1-ITMX [O1, O2] \\
\hline
ITM05 & 60 & $\approx$ 200  & 0 & 0 &  & Spare at CIT \\
\hline
ITM10 & 60 & $\approx$ 300  & 0 & 0 &  & Spare at CIT \\
\hline
ITM01 & 60 & $\approx$ 200  & 0 & 0 &  & Spare at CIT \\
\hline
ITM09 & 60 & $\approx$ 200  & 0 & 0 &  & 3ifo at CIT \\
\hline
ITM06 & 60 & $\approx$ 200  & 0 & 0 &  & 3ifo at CIT \\
\hline \hline
ETM08 & 100 & $\approx$ 500  & 1 & $\approx$ 1000  &  Further measurement at defects in transmittance map identified two absorption points, 33 and 23 ppm & H1-ETMX [O1,O2] \\
\hline
ETM14 & 120 & $\approx$ 90  & 2 & 6000  & Result of a high resolution scan. Max abs. \SI{60}{\micro\meter} beam & 3ifo at CIT \\
\hline
ETM11 & 120 & $\approx$ 60  & 7 & 38400  & Result of a high resolution scan. Max abs. \SI{60}{\micro\meter} beam & 3ifo at CIT \\
\hline
\end{tabular}
\label{tab:PCI}
\caption{Summary of coating absorption measurements from photothermal common-path interferometry.}
\end{table*}
